# Supplementary material for: Probing confined vortices with a superconducting nanobridge
Source: arXiv:2306.01555 source file (2023-06-02)
Supplement: Supplementary file 1 [file Supplemental_Material_to_Probing_confined_vortices.pdf]

# "Probing confined vortices with a superconducting nanobridge" Supplemental Material

M. Foltyn,[1*] K. Norowski,[1] M.J. Wyszyński,[2] A.S. de Arruda,[3]
M.V. Milošević,[2,3*] M. Zgirski,[1*]

[1]Institute of Physics, Polish Academy of Sciences,
Aleja Lotnikow 32/46, PL 02668 Warsaw, Poland,
[2]Department of Physics & NANOlab Center of Excellence,
University of Antwerp, Groenenborgerlaan 171, B-2020 Antwerp, Belgium
[3]Instituto de Física, Universidade Federal de Mato Grosso,
78060-900 Cuiabá, Mato Grosso, Brazil

*To whom correspondence should be addressed:
E-mail: foltyn@ifpan.edu.pl, milorad.milosevic@uantwerpen.be, zgirski@ifpan.edu.pl.

## 1 Main parameters and SEM images of the investigated nanostructures

| Sample | Box size $W$ (nm) | thickness (nm) | Nanobridge length (nm) | Nanobridge width (nm) | Leads width (nm) | $I_{SW}$ ($\mu$A) at 400 mK | Chip[†] |
|---|---|---|---|---|---|---|---|
| **A** (Double box) | 860 | 30 | 195 | 55 | 310 | 50.7 | 1 |
| **B** (Single box) | 860 | 30 | 220 | 45 | 320 | 21.9 | 1 |
| **C** (Single box) | 980 | 30 | 200 | 40 | 245 | 22.5 | 2 |
| **D** (Double box) | 1050 | 30 | 140 | 40 | 285 | 29.7 | 3 |
| **E** (Nanostripe) | - | 30 | 300 | 60 | 540 | 58 | 4 |
| **F** (Nanostripe) | - | 30 | 210 | 70 | 600 | 45 | 5 |

[†]We could prepare several samples on the same silicon chip. If two samples are labelled as made on the same chip, it means that they were made using one same lithography and evaporation process.

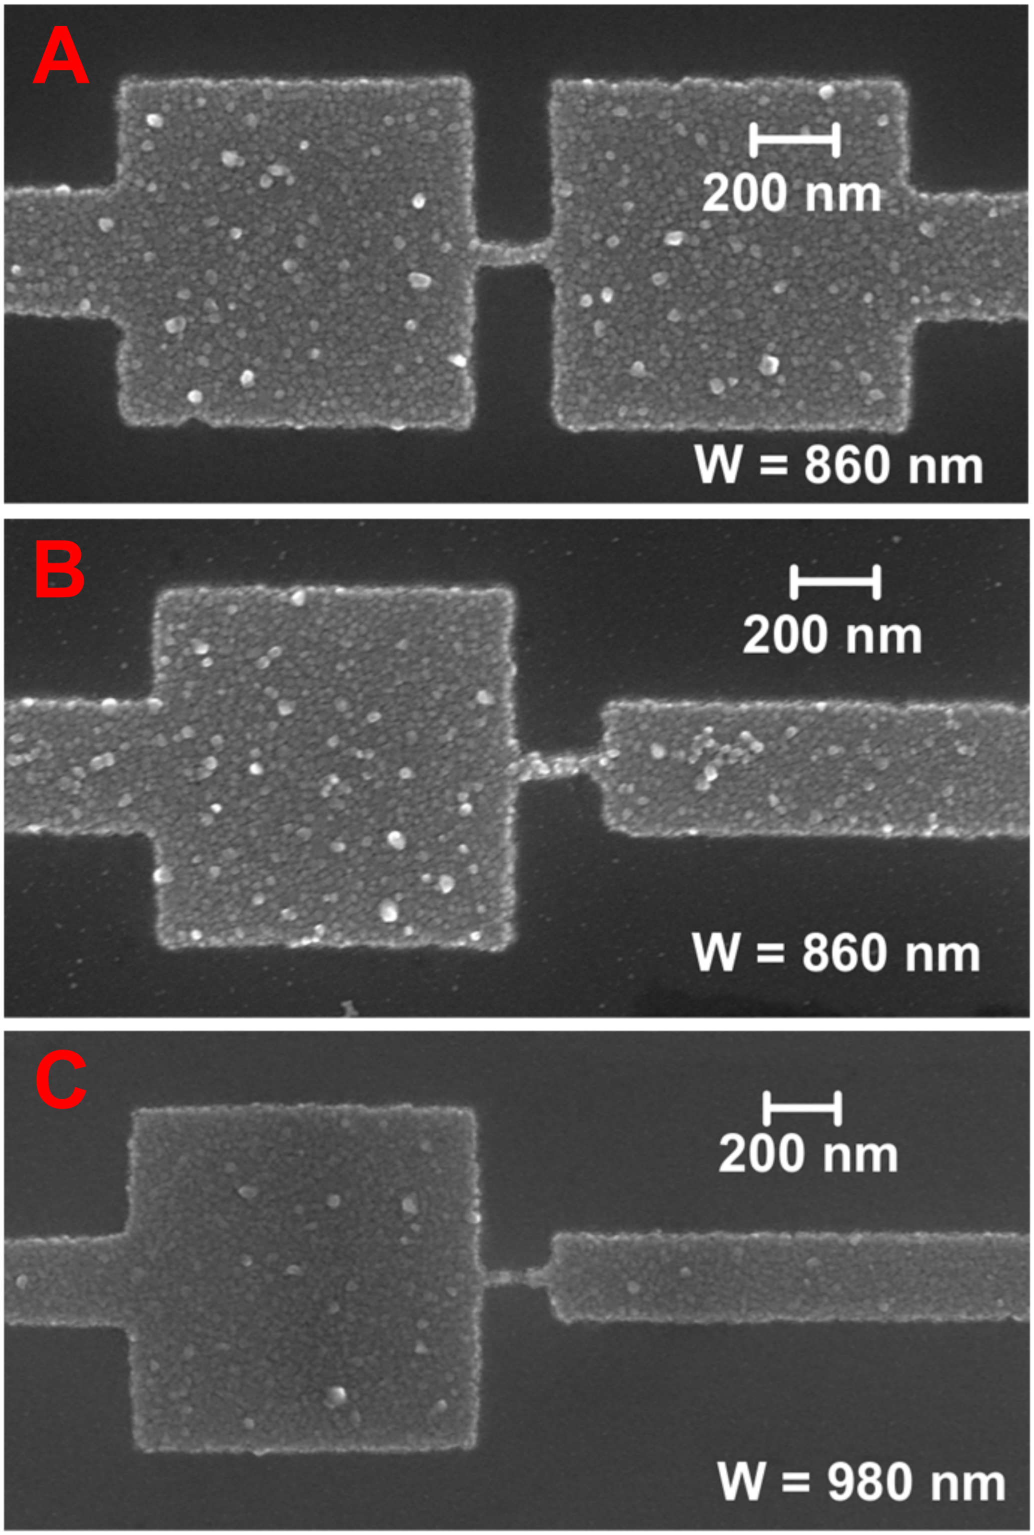


**Figure S1:** The SEM images of samples A-C.

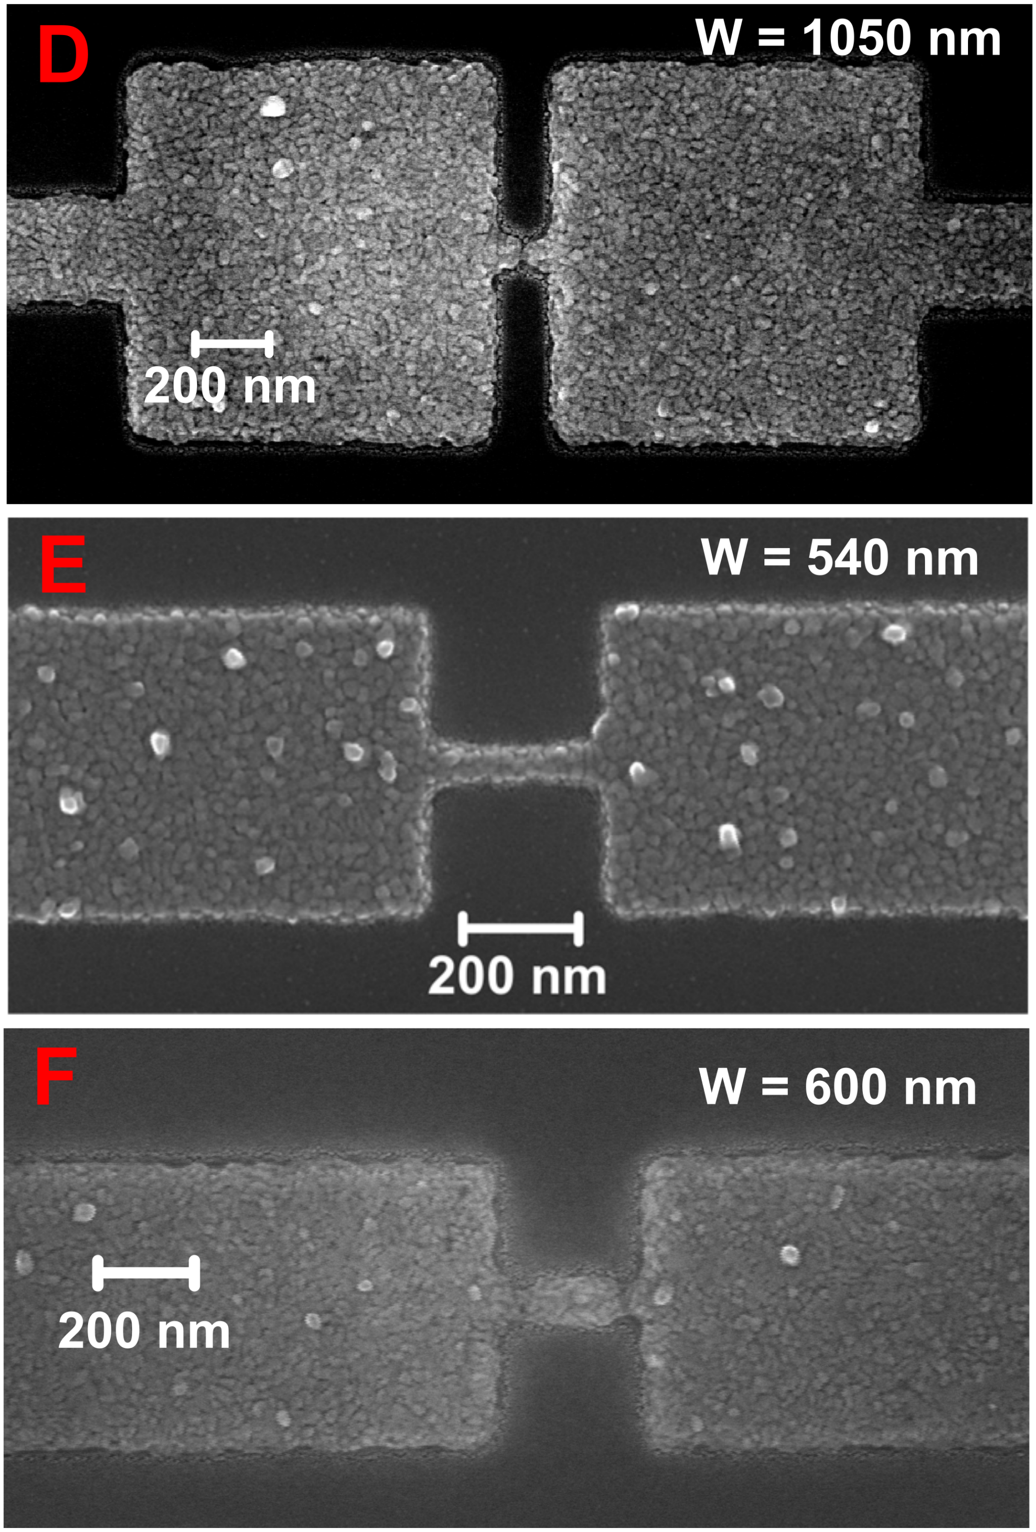


**Figure S2:** The SEM images of samples D-F.

# 2 The dependence of the slope of $I_{SW}(B)$ on coherence length and nanobridge width

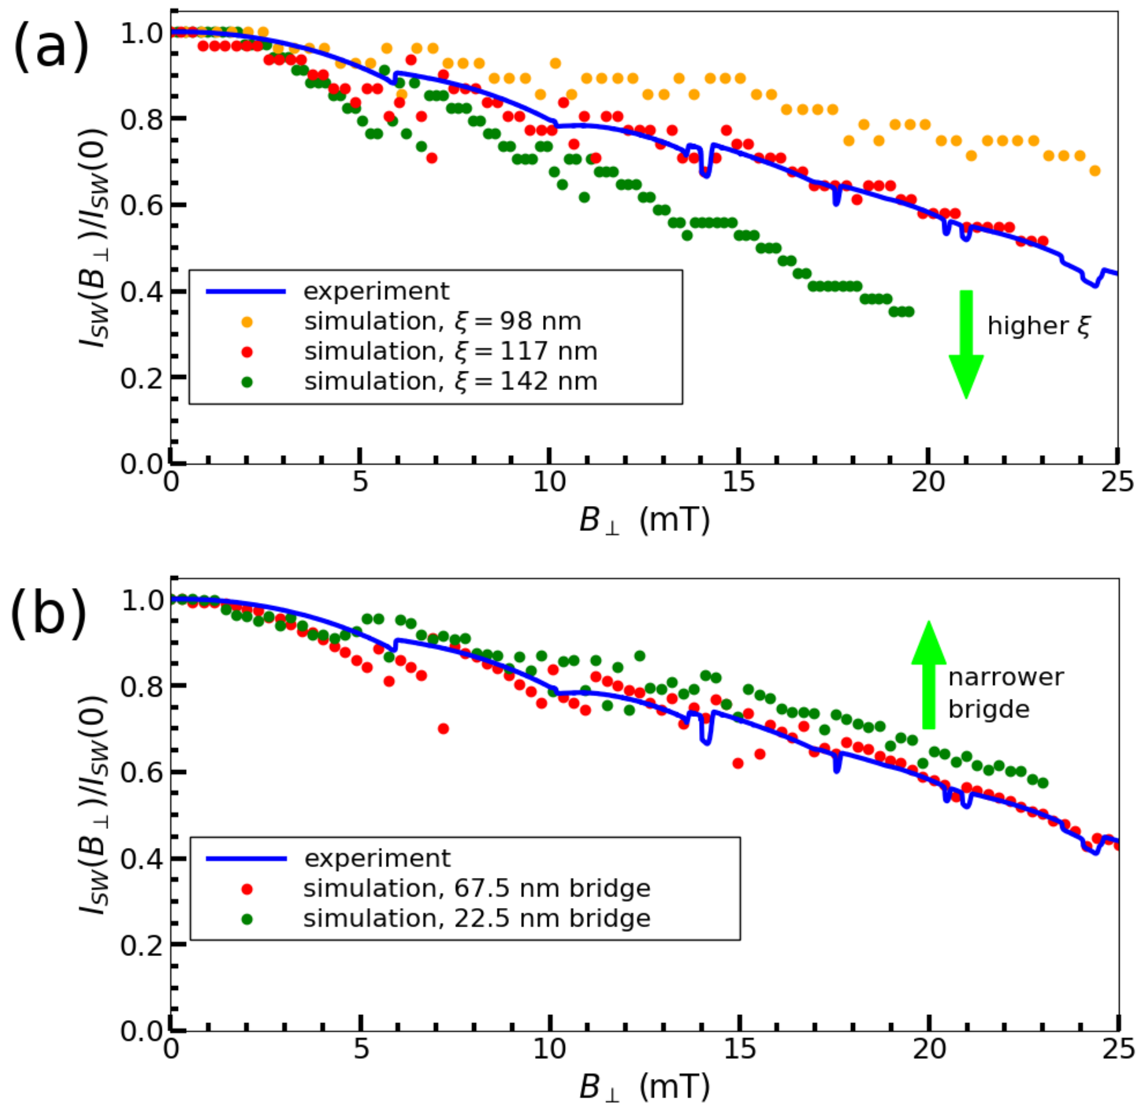


**Figure S3:** $I_{SW}(B)$ dependence on the two fitting parameters for tdGL simulations of sample A. In panel (a), the bridge width was fixed at 67.5 nm and coherence length $\xi(T = 0)$ was varied. In panel (b), $\xi(T = 0)$ was fixed at 117 nm and the width of nanobridge was varied. The solid line shows experimental data recorded for sample A.

# 3 Simulated data for samples B and C

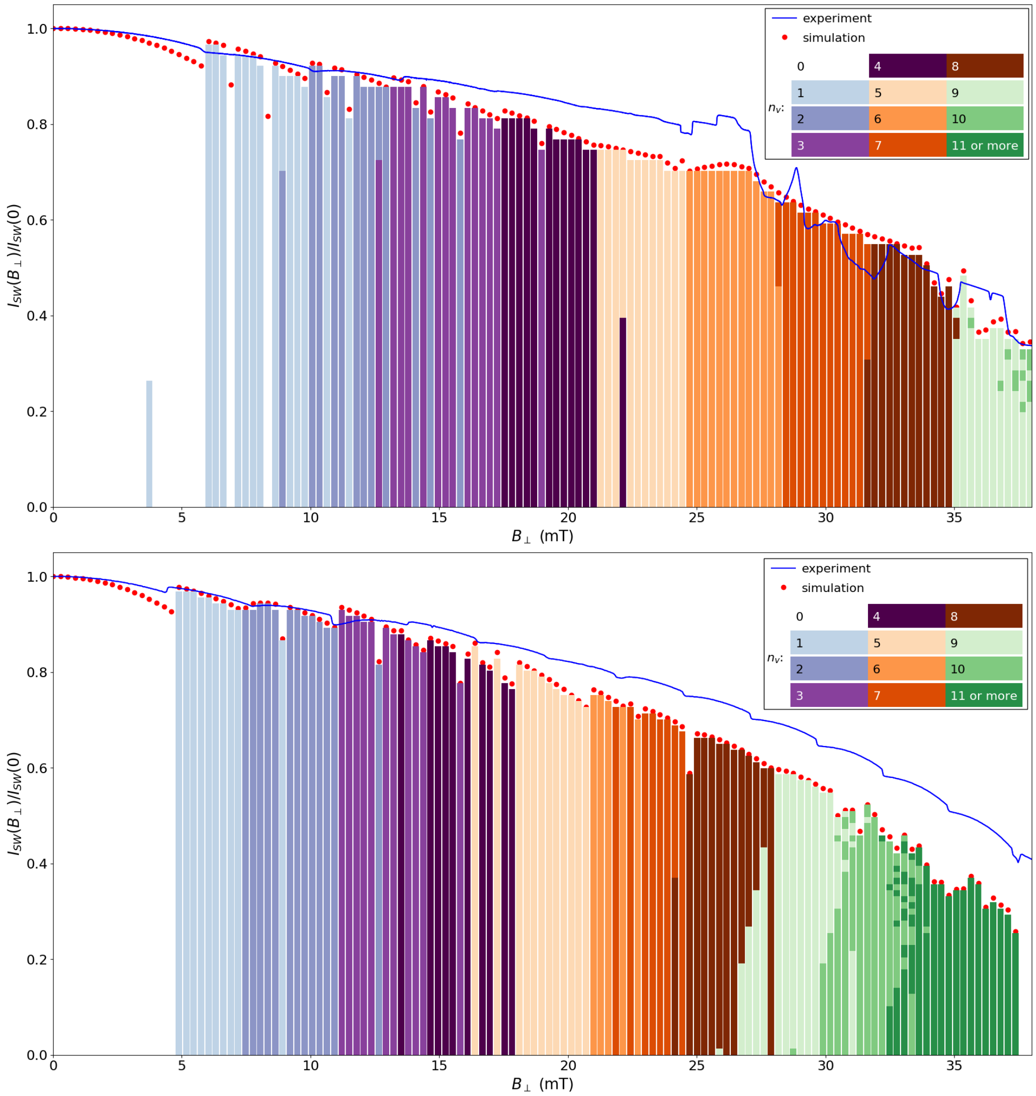


**Figure S4:** Normalized critical current versus the perpendicular applied magnetic field for samples B and C, obtained with tdGL simulations (red points) and corresponding experimental data (blue lines), measured at bath temperature $T_0 = 400$ mK. By lowering the coherence length $\xi$ by a reasonable fraction we could obtain the simulated curves which are closer to the experimental data [see Fig. S3(a)] for the effect of $\xi$ on the calculated $I_{SW}(B)$ traces, but we deliberately chose the same $\xi$(400 mK)=128 nm as for sample A (see Fig. 4 of the main text).

# 4 Detailed switching current $I_{SW}$ vs. the perpendicular magnetic field $B_\perp$ for selected samples

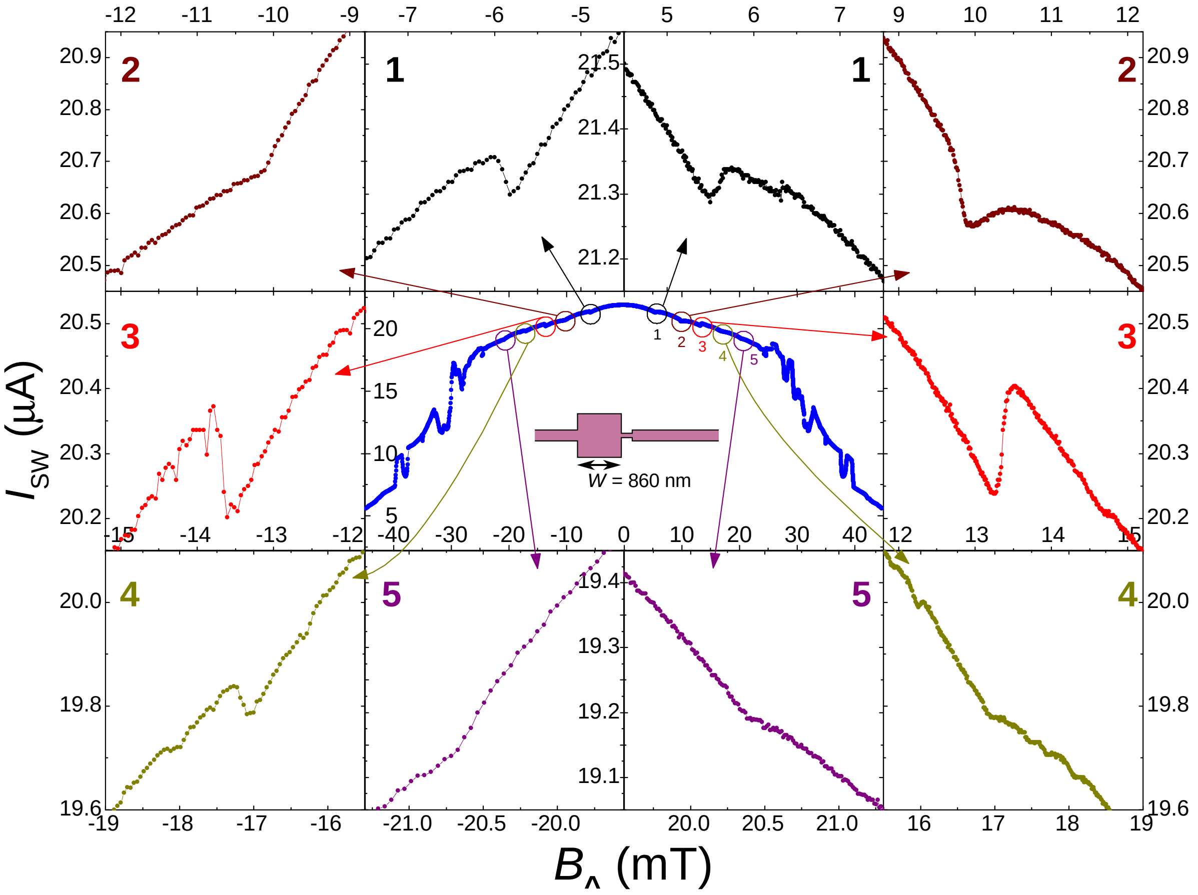


**Figure S5:** $I_{SW}$ vs. $B_\perp$ for sample B, measured at bath temperature $T_0 = 400$ mK.

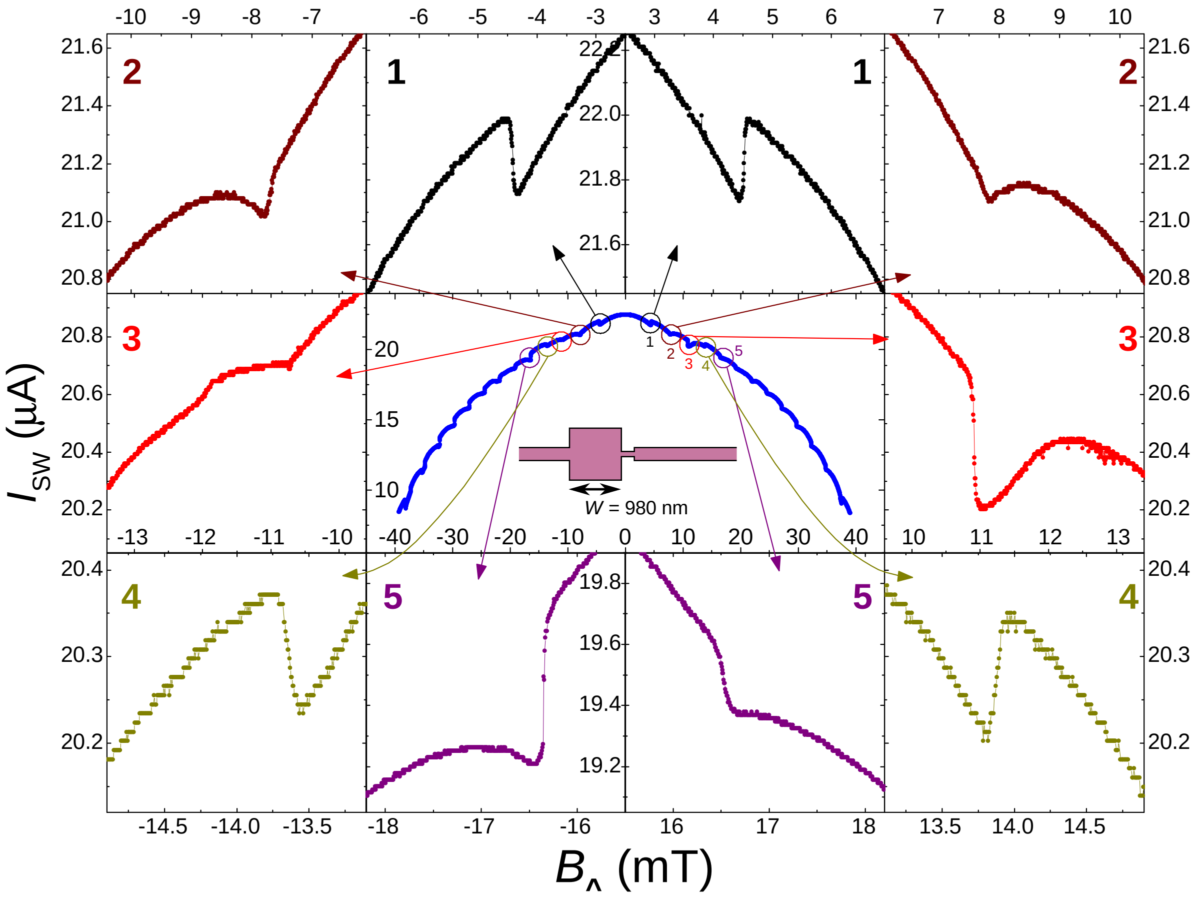


**Figure S6:** $I_{SW}$ vs. $B_\perp$ for sample C, measured at bath temperature $T_0 = 400$ mK.

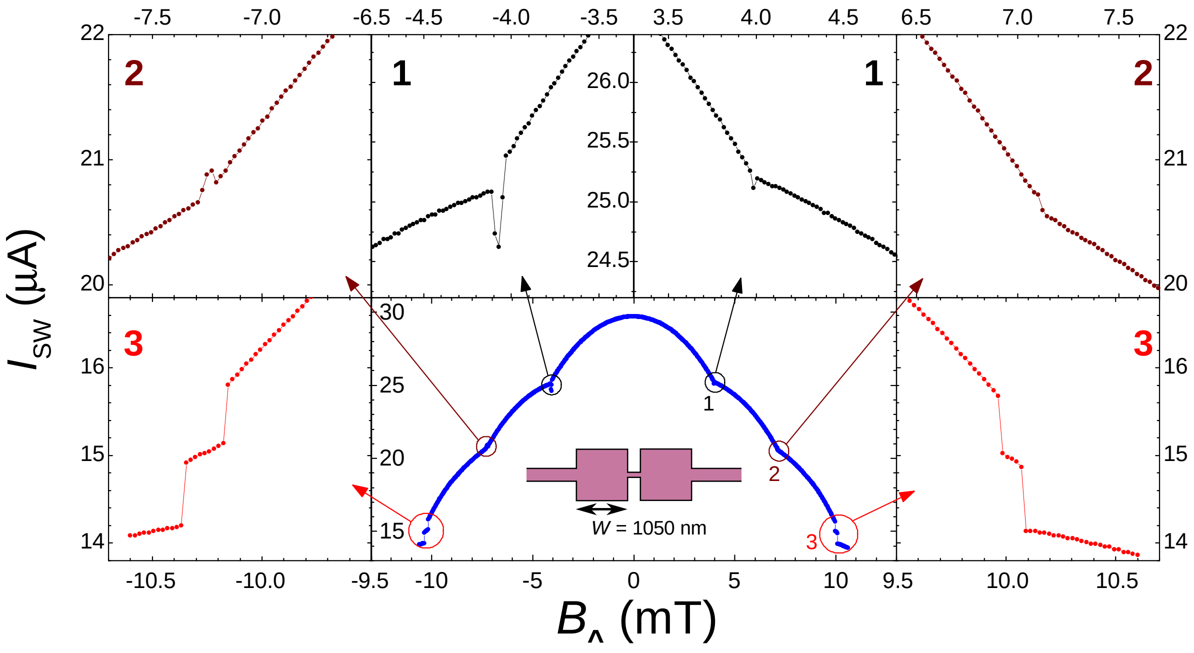


**Figure S7:** $I_{SW}$ vs. $B_\perp$ for sample D, measured at bath temperature $T_0 = 400$ mK.
